# Supplementary material for: Resilient Sensor Fusion under Adverse Sensor Failures via Multi-Modal Expert Fusion
Source: arXiv:2503.19776 source file (2025-03-31)
Supplement: Supplementary file 1 [file table_supple_5.tex]

\begin{table*}[!h]
    \centering
    \tiny
    \setlength{\tabcolsep}{3pt}
    
    \setlength{\arrayrulewidth}{0.3pt}
    % (a) Limited FOV table
    \begin{tabular}{@{}c|cc|cc|cc|cc|cc|cc@{\hspace{4pt}}}
       \toprule[0.1pt]
       \multirow{2}{*}[-2pt]{\tiny \hspace{2pt} Method} & \multicolumn{2}{c|}{Limited FOV} & \multicolumn{2}{c|}{Limited FOV} & \multicolumn{2}{c|}{Limited FOV} & \multicolumn{2}{c|}{Limited FOV} & \multicolumn{2}{c|}{Limited FOV} & \multicolumn{2}{c}{Limited FOV} \\ 
        
        \multicolumn{1}{c|}{} & \multicolumn{2}{c|}{\textit{[-180, 180]}} & \multicolumn{2}{c|}{\textit{[-150, 150]}} & \multicolumn{2}{c|}{\textit{[-120, 120]}} & \multicolumn{2}{c|}{\textit{[-90, 90]}} & \multicolumn{2}{c|}{\textit{[-60, 60]}} & \multicolumn{2}{c}{\textit{[-30, 30]}} \\
        \cline{2-13}
        & mAP & NDS & mAP & NDS & mAP & NDS & mAP & NDS & mAP & NDS & mAP & NDS \\ 
        \hline
        \hspace{2pt} CMT~\cite{cmt} & 70.3 & 72.9 & 65.4 & 69.8 & 53.8 & 62.2 & 49.0 & 58.4 & 43.9 & 54.0 & 35.0 & 46.1 \\
        \textbf{ \hspace{2pt} Immortal (ours)} & \textbf{71.2} & \textbf{73.6} & \textbf{67.8} & \textbf{71.2} & \textbf{56.2} & \textbf{63.4} & \textbf{54.2} & \textbf{61.2} & \textbf{50.6} & \textbf{58.3} & \textbf{44.0} & \textbf{53.0} \\ 
        \bottomrule[0.01pt]
    \end{tabular}
    \vspace{1em}
    
    % (b) Object Failure table
    \begin{tabular}{@{}c|cc|cc|cc|cc|cc|cc@{\hspace{4pt}}}
       \toprule[0.1pt]
       \multirow{2}{*}[-2pt]{\tiny \hspace{2pt} Method} & \multicolumn{2}{c|}{Object Failure} & \multicolumn{2}{c|}{Object Failure} & \multicolumn{2}{c|}{Object Failure} & \multicolumn{2}{c|}{Object Failure} & \multicolumn{2}{c|}{Object Failure} & \multicolumn{2}{c}{Object Failure} \\ 
        
        \multicolumn{1}{c|}{} & \multicolumn{2}{c|}{\textit{ratio=0.0}} & \multicolumn{2}{c|}{\textit{ratio=0.1}} & \multicolumn{2}{c|}{\textit{ratio=0.3}} & \multicolumn{2}{c|}{\textit{ratio=0.5}} & \multicolumn{2}{c|}{\textit{ratio=0.7}} & \multicolumn{2}{c}{\textit{ratio=0.9}} \\
        \cline{2-13}
        & mAP & NDS & mAP & NDS & mAP & NDS & mAP & NDS & mAP & NDS & mAP & NDS \\ 
        \hline
        \hspace{2pt} CMT~\cite{cmt} & 54.9 & 62.2 & 38.3 & 44.7 & 43.9 & 54.0 & 66.7 & 70.4 & 61.7 & 68.1 & 57.8 & 65.3 \\
        \textbf{ \hspace{2pt} Immortal (ours)} & \textbf{55.0} & \textbf{63.0} & \textbf{42.5} & \textbf{48.2} & \textbf{50.6} & \textbf{58.3} & \textbf{67.0} & \textbf{71.0} & \textbf{63.6} & \textbf{69.5} & \textbf{60.2} & \textbf{67.1} \\ 
        \bottomrule[0.01pt]
    \end{tabular}
    \vspace{1em}
    
    % (c) Beam Reduction table
    \begin{tabular}{@{}c|cc|cc|cc|cc|cc|cc@{\hspace{4pt}}}
       \toprule[0.1pt]
       \multirow{2}{*}[-2pt]{\tiny \hspace{2pt} Method} & \multicolumn{2}{c|}{Beam Reduction} & \multicolumn{2}{c|}{Beam Reduction} & \multicolumn{2}{c|}{Beam Reduction} & \multicolumn{2}{c|}{Beam Reduction} & \multicolumn{2}{c|}{Beam Reduction} & \multicolumn{2}{c}{Beam Reduction} \\ 
        
        \multicolumn{1}{c|}{} & \multicolumn{2}{c|}{\textit{1 beams}} & \multicolumn{2}{c|}{\textit{4 beams}} & \multicolumn{2}{c|}{\textit{8 beams}} & \multicolumn{2}{c|}{\textit{16 beams}} & \multicolumn{2}{c|}{\textit{24 beams}} & \multicolumn{2}{c}{\textit{32 beams}} \\
        \cline{2-13}
        & mAP & NDS & mAP & NDS & mAP & NDS & mAP & NDS & mAP & NDS & mAP & NDS \\ 
        \hline
        \hspace{2pt} CMT~\cite{cmt} & 54.9 & 62.2 & 38.3 & 44.7 & 43.9 & 54.0 & 61.7 & 68.1 & 63.2 & 69.4 & 64.5 & 70.2 \\
        \textbf{ \hspace{2pt} Immortal (ours)} & \textbf{55.0} & \textbf{63.0} & \textbf{42.5} & \textbf{48.2} & \textbf{50.6} & \textbf{58.3} & \textbf{63.6} & \textbf{69.5} & \textbf{65.4} & \textbf{70.8} & \textbf{66.8} & \textbf{71.8} \\ 
        \bottomrule[0.01pt]
    \end{tabular}
    \vspace{1em}
    
    % (d) View Drop table
    \begin{tabular}{@{}c|cc|cc|cc|cc|cc|cc@{\hspace{4pt}}}
       \toprule[0.1pt]
       \multirow{2}{*}[-2pt]{\tiny \hspace{2pt} Method} & \multicolumn{2}{c|}{View Drop} & \multicolumn{2}{c|}{View Drop} & \multicolumn{2}{c|}{View Drop} & \multicolumn{2}{c|}{View Drop} & \multicolumn{2}{c|}{View Drop} & \multicolumn{2}{c}{View Drop} \\ 
        
        \multicolumn{1}{c|}{} & \multicolumn{2}{c|}{\textit{1 drop}} & \multicolumn{2}{c|}{\textit{2 drops}} & \multicolumn{2}{c|}{\textit{3 drops}} & \multicolumn{2}{c|}{\textit{4 drops}} & \multicolumn{2}{c|}{\textit{5 drops}} & \multicolumn{2}{c}{\textit{6 drops}} \\
        \cline{2-13}
        & mAP & NDS & mAP & NDS & mAP & NDS & mAP & NDS & mAP & NDS & mAP & NDS \\ 
        \hline
        \hspace{2pt} CMT~\cite{cmt} & 54.9 & 62.2 & 38.3 & 44.7 & 43.9 & 54.0 & 66.7 & 70.4 & 61.7 & 68.1 & 58.2 & 66.5 \\
        \textbf{ \hspace{2pt} Immortal (ours)} & \textbf{55.0} & \textbf{63.0} & \textbf{42.5} & \textbf{48.2} & \textbf{50.6} & \textbf{58.3} & \textbf{67.0} & \textbf{71.0} & \textbf{63.6} & \textbf{69.5} & \textbf{61.7} & \textbf{68.1} \\ 
        \bottomrule[0.01pt]
    \end{tabular}

    \caption{Experimental comparisons on sensor corruptions with various degrees. (a) Limited FOV shows influence of reduced field of view, (b) Object Failure demonstrates robustness under varying object detection failures, (c) Beam Reduction evaluates performance with different LiDAR beam configurations, and (d) View Drop tests resilience against camera view losses. Our Immortal consistently outperforms CMT across all corruption settings.}
\label{table:sensor_corruptions}
\end{table*}
